# Supplementary material for: Individual Rationality Conditions of Identifying Matching Costs in Transferable Utility Matching Games
Source: arXiv:2204.00713 source file (2024-05-07)
Supplement: Supplementary file 1 [file 02supplement_identification_region_plot.tex]

The parameter $\beta$ is estimated as a maximizer or a set of maximizers of $Q(\beta)$ or $\tilde{Q}(\beta)$ so that $\beta$ lie within a high-dimensional polytope determined by inequalities in Table \ref{tb:num_inequalities}. Although it is difficult to show the general case, I show what type of inequality corresponds with a hyperplane restricting identified set of $\beta$ in Section \ref{subsec:supplement_identification_region_plot}.

To illustrate the restriction power of inequalities, I introduce a simple example. Let $\mathcal{M}_{b}^m=\{1,2\}$, $\mathcal{M}_{b}^u=\{3\}$, $\mathcal{M}_{s}^m=\{a,b\}$, and $\mathcal{M}_{s}^u=\{c\}$. Suppose that I observe matched pairs $(1,a)$ and $(2,b)$ and unmatched pairs $(3,\emptyset)$ and $(\emptyset,c)$. I specify the total matching value $f(b,s)=1\cdot \bar{X}_{b,s}+X_{b,s}\beta$ where $1$ is a normalized constant parameter, $\beta\in\mathbb{R}$, two dimensional match-specific observed characteristic $(\bar{X}_{b,s},X_{b,s})\in\mathbb{R}\times \mathbb{R}$, and $p_{b,s}$ is a transfer for matches $(b,s)$. When transfer data is available, by Table \ref{tb:num_inequalities}, reserachers can construct $_4C_3=12$ inequalities. Our objective is to find the set of $\beta$ which satisfies all inequalities summarized as:
\begin{align}
    \begin{cases}
         f(1, a)-f(1, b) \geq p_{1 a}-p_{1 b} \\
f(1, a)-f(1, c) \geq p_{1 a}-p_{1 c} \\
f(1, a)-f(1, \emptyset) \geq p_{1 a}-p_{1\emptyset} \\
f(2, b)-f(2, a) \geq p_{2 b}-p_{2 a} \\
f(2, b)-f(2, c) \geq p_{2 b}-p_{2 c} \\
f(2, b)-f(2, \emptyset) \geq p_{2 b}-p_{2\emptyset} \\
f(3, \emptyset)-f(3, a) \geq p_{3 \emptyset}-p_{3 a} \\
f(3, \emptyset)-f(3, b) \geq p_{3\emptyset}-p_{3 b} \\
f(3, \emptyset)-f(3, c) \geq p_{3 \emptyset}-p_{3 c}\\
f(\emptyset, c)-f(1, c) \geq p_{\emptyset,c}-p_{1 c} \\
f(\emptyset, c)-f(2, c) \geq p_{\emptyset,c}-p_{2 c} \\
f(\emptyset, c)-f(3, c) \geq p_{\emptyset,c}-p_{3 c}
    \end{cases}
\rightarrow \begin{cases}
    (\bar{X}_{1a}-\bar{X}_{1b})+(X_{1a}-X_{1b})\beta \ge p_{1a}-p_{2b}\\
    (\bar{X}_{1a}-\bar{X}_{1c})+(X_{1a}-X_{1c})\beta \ge p_{1a}-p_{1c}\\
    \bar{X}_{1a}+X_{1a}\beta \ge p_{1a}\\
    (\bar{X}_{2b}-\bar{X}_{2a})+(X_{2b}-X_{2a})\beta \ge p_{2b}-p_{1a}\\
    (\bar{X}_{2b}-\bar{X}_{2c})+(X_{2b}-X_{2c})\beta \ge p_{2b}-p_{2c}\\
    \bar{X}_{2b}+X_{2b}\beta \ge p_{2b}\\
    \bar{X}_{3a}+X_{3a}\beta \le p_{3a}\le p_{1a}\\
    \bar{X}_{3b}+X_{3b}\beta \le p_{3b}\le p_{2b}\\
    \bar{X}_{3c}+X_{3c}\beta \le p_{3c}= 0 \\
    \bar{X}_{1c}+X_{1c}\beta \le p_{1c}\\
    \bar{X}_{2c}+X_{2c}\beta \le p_{2c}\\
    \bar{X}_{3c}+X_{3c}\beta \le p_{3c}= 0 
\end{cases},\label{eq:example_all_ineq}
\end{align}
where I substitute $p_{2b}\ge p_{1b}$, $p_{1a}\ge p_{2a}$, and $p_{3c}= 0$ under the equilibrium price property as in \cite{akkus2015ms}.

Suppose that the researchers do not have data about transfers but unmatched firms. Then, by Table \ref{tb:num_inequalities}, they can construct $\frac{1}{2}\cdot 4 \cdot 3=6$ inequalities as: 

\begin{align}
    \begin{cases}
f(1, a) + f(2, b) \geq f(1, b)+f(2, a) \\
f(1, a) + f(3, \emptyset) \geq f(1,\emptyset) + f(3, a)\\
f(2, b) + f(3, \emptyset) \geq f(2, \emptyset) + f(3, b)\\
f(1, a) + f(\emptyset, c) \geq f(1, c)+f(\emptyset, a) \\
f(2, b) + f(\emptyset, c) \geq f(2, c) + f(\emptyset, b)\\
f(3, \emptyset) + f(\emptyset, c) \geq f(3, c) + f(\emptyset, \emptyset)
\end{cases}\rightarrow \begin{cases}
    (\bar{X}_{1a}+\bar{X}_{2b}-\bar{X}_{1b}-\bar{X}_{2a})+(X_{1a}+X_{2b}-X_{1b}-X_{2a})\beta \ge 0\\
    (\bar{X}_{1a}-\bar{X}_{3a})+(X_{1a}-X_{3a})\beta \ge 0\\
    (\bar{X}_{2b}-\bar{X}_{3b})+(X_{2b}-X_{3b})\beta \ge 0\\
    (\bar{X}_{1a}-\bar{X}_{1c})+(X_{1a}-X_{1c})\beta \ge 0\\
    (\bar{X}_{2b}-\bar{X}_{2c})+(X_{2b}-X_{2c})\beta \ge 0\\
    0 \ge \bar{X}_{3c}+X_{3c}\beta.
\end{cases}\label{eq:num_ineq_without_transfer}
\end{align}

Suppose that the researchers do not have data about unmatched firms but transfers. Then, by Table \eqref{tb:num_inequalities}, they can construct $2$ inequalities as: 
\begin{align}
    \begin{cases}
f(1, a)-f(1, b) \geq p_{1 a}-p_{1 b} \\
f(2, b)-f(2, a) \geq p_{2 b}-p_{2 a} 
\end{cases}\rightarrow \begin{cases}
    (\bar{X}_{1a}-\bar{X}_{1b})+(X_{1a}-X_{1b})\beta \ge p_{1a}-p_{2b}\\
    (\bar{X}_{2b}-\bar{X}_{2a})+(X_{2b}-X_{2a})\beta \ge p_{2b}-p_{1a}.
\end{cases}\label{eq:num_ineq_without_unmatched}
\end{align}

Suppose that the researchers do not have data about transfers and unmatched firms. Then, by Table \eqref{tb:num_inequalities}, they can construct $1$ inequality as: 
\begin{align}
    &\begin{array}{l}
f(1, a) + f(2, b) \geq f(1, b)+f(2, a) 
\end{array}\nonumber\\
     &\rightarrow \begin{array}{l}
    (\bar{X}_{1a}+\bar{X}_{2b}-\bar{X}_{1b}-\bar{X}_{2a})+(X_{1a}+X_{2b}-X_{1b}-X_{2a})\beta \ge 0.
\end{array}\label{eq:num_ineq_without_transfer_and_unmatched}
\end{align}

Note that the set of inequalities \eqref{eq:num_ineq_without_unmatched} is a strict subset of inequalities \eqref{eq:example_all_ineq} and the set of the inequalities \eqref{eq:num_ineq_without_transfer_and_unmatched} is a strict subset of inequalities \eqref{eq:num_ineq_without_transfer}. Thus, monotonicity of the sets of equilibrium constraints indicates that the identification power decreases as \eqref{eq:example_all_ineq} is replaced with \eqref{eq:num_ineq_without_unmatched} and \eqref{eq:num_ineq_without_transfer} is replaced with \eqref{eq:num_ineq_without_transfer_and_unmatched}. Thus, I only need to show that the identification power decreases as inequalities \eqref{eq:example_all_ineq} is replaced with inequalities \eqref{eq:num_ineq_without_transfer}. Formally, I need to compare
\begin{align*}
    \begin{array}{l}
    \begin{cases}
         (\bar{X}_{1a}-\bar{X}_{1b})+(X_{1a}-X_{1b})\beta \ge p_{1a}-p_{2b}\\
         (\bar{X}_{2b}-\bar{X}_{2a})+(X_{2b}-X_{2a})\beta \ge p_{2b}-p_{1a}
    \end{cases}
\end{array}\text{and}\quad
\begin{array}{l}
    (\bar{X}_{1a}+\bar{X}_{2b}-\bar{X}_{1b}-\bar{X}_{2a})\\
    \quad\quad\quad+(X_{1a}+X_{2b}-X_{1b}-X_{2a})\beta \ge 0,
\end{array}
\end{align*}
since the other inequalities in \eqref{eq:example_all_ineq} are analogously derived. Let the comparison be denoted concisely as:
\begin{align*}
    \begin{array}{l}
    \begin{cases}
         A+B\beta \ge C\\
         D+E\beta \ge -C
    \end{cases}
\end{array}\text{and}\quad (A+D)+(B+E)\beta \ge 0.
\end{align*}
Without of loss generality, assume $C>0$. Then, the inequalities are expressed as
\begin{align}
    \begin{array}{l}
    \begin{cases}
         \beta \ge \frac{C-A}{B}\\
         \frac{C+D}{-E} \ge \beta
    \end{cases}
\end{array}\text{and}\quad \beta \ge \frac{-(A+D)}{(B+E)}.\label{eq:ineq_concise}
\end{align}
Whenever $\frac{C+D}{-E}\ge \frac{C-A}{B}$ or $\frac{C+D}{-E}\le \frac{C-A}{B}$, the left equations can be bounded by the two composite terms.

To illustrate the power of inequality restrictions for each inequality, I fix some elements determined by data. Assume that $C=1$ and $A=D=0$, i.e., the first observed characteristic has no effect on the inequalities. Then, \eqref{eq:ineq_concise} is reduced to
\begin{align*}
    \begin{array}{l}
    \begin{cases}
         \beta \ge \frac{1}{B}\\
         \frac{1}{-E} \ge \beta
    \end{cases}
\end{array}\text{and}\quad (B+E)\beta \ge 0.
\end{align*}
I denote the left equations as \textit{separated inequalities} and the right equation as \textit{composite inequality}. Also, I denote $\beta \le \frac{-\bar{X}_{3c}}{X_{3c}}$ derived from the ninth line of inequalities \eqref{eq:example_all_ineq} as \textit{unmatched inequality} and fix constant $\frac{-\bar{X}_{3c}}{X_{3c}}=5$.

Figure \ref{fg:identification_region_3d} illustrates the upper and lower bounds of $\beta$ induced by separated inequalities (red and blue), lower bound of $\beta$ induced by composite inequality (green), and upper bound of the unmatched inequality (yellow). Note that the $\beta$ in the composite inequality is upper unbounded for each matching pair. The figure focuses only on the domains (the case of $B>0, E>0$ and the case of $B>0, E<0$), however, the other domains can be analogously illustrated. First, I find that the identification power decreases when inequalities \eqref{eq:example_all_ineq} is reduced to inequalities \eqref{eq:num_ineq_without_transfer} because the identification set derived from the composite inequality is much larger than the identification set derived from the separated inequalities. Second, the identification set shrinks as $B$ and $E$ is larger. This means that the differences of match-specific characteristics between the observed match and swapped match help identification of $\beta$ significantly. Third, unmatched inequality help identification significantly especially when $B$ and $E$ are close to zero, i.e., the differences of match-specific characteristics between the observed match and swapped match are small.

In the above simple example, I find how each type of inequality in each matching pair characterizes the identified set of $\beta$. In the general model, the identified set is characterized as a polytope. In Section \ref{sec:simulation_bound}, I investigate how each type of inequality contributes to the identification totally through the objective function of the matching maximum score estimator.

\begin{figure}[htbp]
  \begin{minipage}{0.5\hsize}
  \begin{center}
   \includegraphics[width=60mm]{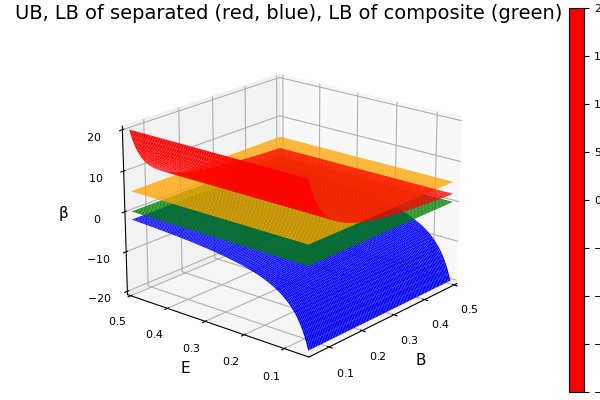}
  \end{center}
 \end{minipage}
 \begin{minipage}{0.5\hsize}
  \begin{center}
   \includegraphics[width=60mm]{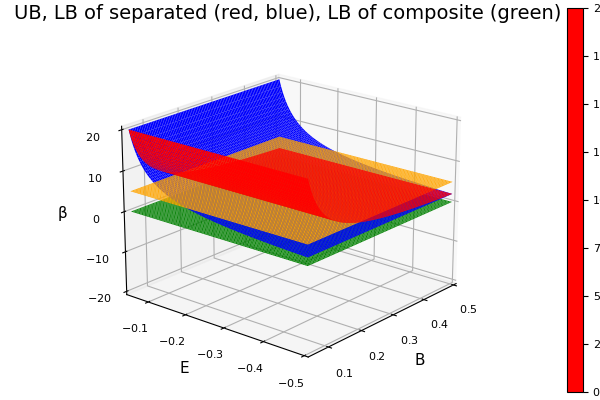}
  \end{center}
 \end{minipage}
 \caption{\textbf{The identification power of inequalities for each matching pair}. Fix $C=1$ and $A=D=0$. The domains of left and right panels are restricted to ($B>0,E>0$) and ($B>0,E<0$) respectively. The red and blue surfaces mean the upper and lower bounds of parameter $\beta$ derived from the separated inequality in inequalities \eqref{eq:ineq_concise}. The roles of bounds are reversed in some domains in the right panel. The green surface means the lower (or upper) bounds of parameter $\beta$ derived from the composite inequality in inequalities \eqref{eq:ineq_concise}. The yellow surface means the upper bound of parameter $\beta$ derived from unmatched inequality and fixed to $5$.}
\label{fg:identification_region_3d}
\end{figure}
